# Supplementary material for: U.S. State Guidance on AI in K-12 Education: A Comparative Content and Citation Analysis
Source: arXiv:2611.06762 source file (2026-11-04)
Supplement: Supplementary file 1 [file rq3_appendix_tables.tex]

% Paste into the appendix, e.g. after "Data sources for RQ2". These two tables moved out of Section 3.
\subsection{Epistemic sources for RQ3}
\begin{table}[h]
\centering
\small
\begin{tabular}{p{3.0cm}p{8.0cm}r}
\toprule
\textbf{Pass} & \textbf{What is searched} & \textbf{Hits} \\
\midrule
1. Hyperlinks & Link annotations and printed web addresses, matched by website & 3{,}993 \\
2. Named sources & About 130 sources, by name pattern & 2{,}556 \\
3. Peer-state mentions & State name or agency acronym near a word such as ``Department'' or ``guidance'', in an AI passage & 189 \\
\midrule
Total & & 6{,}738 \\
\bottomrule
\end{tabular}
\caption{Hits returned by each search pass, before removing hits that are not outside sources.}
\label{tab:rq3-channels}
\end{table}

\begin{table}[h]
\centering
\small
\begin{tabular}{p{5.2cm}p{6.6cm}}
\toprule
\textbf{Type} & \textbf{Examples} \\
\midrule
Federal government & U.S.\ Dept.\ of Education, FTC, NIST \\
Other state government & Washington, Oregon, North Carolina \\
Local school district & (excluded from main analysis) \\
International organization & UNESCO, OECD, European Union \\
Advocacy group, nonprofit or union & TeachAI, Code.org, Common Sense Media \\
Professional association & ISTE, CoSN, CSTA \\
Philanthropic foundation & Kapor Foundation, Walton Family Foundation \\
Research institute, think tank or university & Brookings, Stanford HAI, CIRCLS \\
Company or consultancy & Google, Microsoft, OpenAI \\
\midrule
Law or legal requirement$^{\ast}$ & FERPA, COPPA, IDEA \\
Media, reference or other$^{\ast}$ & EdWeek, Common Core \\
\bottomrule
\end{tabular}
\caption{Source types. $^{\ast}$Added by us; the others follow actor kinds in prior work.}
\label{tab:rq3-types}
\end{table}
